# Supplementary material for: Two-dimensional helical superconductivity and gapless superconducting edge modes in the 1T$^\prime$-WS$_2$/2H-WS$_2$ heterophase bilayer
Source: arXiv:2512.10157 source file (2025-12-10)
Supplement: Supplementary file 1 [file WS2_SI.pdf]

# Supplementary Information of "Two-dimensional helical superconductivity and gapless superconducting edge modes in the 1T′-$WS_2$/2H-$WS_2$ heterophase bilayer"

Xuance Jiang,[1,2,*] Jennifer Cano,[2,3] Yuan Ping,[4,5,6] Yafis Barlas,[7,†] and Deyu Lu[1,‡]

[1] *Center for Functional Nanomaterials, Brookhaven National Laboratory, Upton, NY 11973, USA*
[2] *Department of Physics and Astronomy, Stony Brook University, Stony Brook, NY 11794, USA*
[3] *Center for Computational Quantum Physics, Flatiron Institute, New York, New York 10010, USA*
[4] *Department of Materials Science and Engineering, University of Wisconsin-Madison, WI, 53706, USA*
[5] *Department of Physics, University of Wisconsin-Madison, WI, 53706, USA*
[6] *Department of Chemistry, University of Wisconsin-Madison, WI, 53706, USA*
[7] *Department of Physics, University of Nevada, Reno, 1664 N. Virginia Street, Reno, NV 89557, USA*

(Dated: December 9, 2025)

## I. COMPUTATIONAL METHODS

*Ab initio* calculations are performed with the QUANTUM ESPRESSO package [1] using relativistic norm-conserving pseudopotentials within the generalized gradient approximation from Pseudo Dojo [2]. We employ the Perdew-Burke-Ernzerhof exchange-correlation functional [3] with a plane-wave cutoff of 80 Ry and use the DFT-D3 method [4] to treat the van der Waals interactions.

The HPB supercell is constructed by compressing the 1T′-$WS_2$ monolayer by 2% and stretching the 2H-$WS_2$ monolayer by 2%. Then the 1T′-$WS_2$ monolayer is stacked on top of the 2H-$WS_2$ monolayer with the interlayer distance 3 Å. To optimize the relative in-plane translational degree of freedom between two monolayers, we considered two possible ways of stacking, where the 1T′-$WS_2$ monolayer remains the same, but the orientations of the 2H-$WS_2$ monolayer in the two configurations are associated with each other by 180 degree rotation along the out-of-plane direction (Fig. S1a). To find the most stable stacking structure, the formation energy of both configurations was calculated for a series stacking structures with different amount of relative in-plane displacements along the x direction (Fig. S1b). The most stable structure is indicated by the red arrow in configuration 2. The lattice parameters and atomic positions of this most stable structure are fully relaxed until the forces are less than 0.01 eV/Å. The optimized atom positions are listed in Table SI. Results of the analysis of charge transfer and band alignment of the HPB are presented in Fig. S2. The orbital projection of the HPB band structure onto S $p$ orbitals and W $d$ orbitals is shown in Fig. S9.

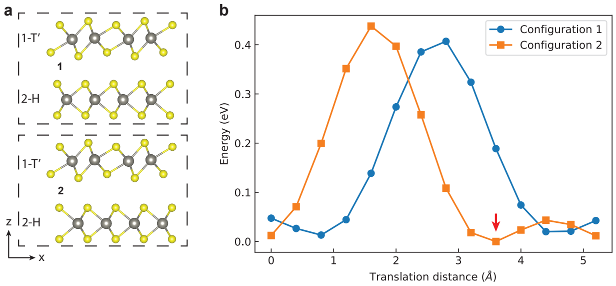


FIG. S1: (a) Two possible configurations of the HPB. Gray and yellow spheres indicate the W and S atoms respectively. (b) Adhesive energy of the HPB model at different relative displacements between two layers along the x direction.

To compute the electron-phonon coupling (EPC), the self-consistent calculations are performed with a Γ-centered 16 x 8 x 1 k-mesh and a Gaussian smearing width of 0.02 Ry. The dynamical matrices and the linear variation of

* xuance@ucsb.edu; Present address: Department of Chemistry and Biochemistry, University of California, Santa Barbara, Santa Barbara, California 93106, USA
Materials Department, University of California, Santa Barbara, Santa Barbara, California 93106, USA
† ybarlas@unr.edu
‡ dlu@bnl.gov

the self-consistent potential are computed within density functional perturbation theory on a 8 x 4 x 1 q-mesh in the absence of SOC. 2D Coloumb interation truncation [5] is applied to eliminate the spurious interaction of in the z direction between periodic images. We use Wannier interpolation on a Γ-centered 16 x 8 x 1 (8 x 4 x 1) grid with 44 maximally localized Wannier functions [6, 7] (5 d orbitals for each W atom and 3 p orbitals for each S atom). With the EPW code [8, 9] , the electron-phonon matrix elements are interpolated onto the 160 x 80 x 1 k- and 80 x 40 x 1 q-point grids to calculate the EPC and $\alpha^2F(\omega)$.

The Fermi pockets and spin projection are plotted using the Wannier Tools package [10] based on the tight-bind model contructed with 44 maximally localized Wannier functions as basis. The edge-mode dispersion is calculated using the same tight-binding model, constructed with 10 finite unit cells along the $x$ direction and periodic boundary conditions along the $y$ direction.

TABLE SI: Lattice parameters and atomic coordinates of the HPB model.

| Lattice parameters ( Å) | | | |
|---|---|---|---|
| $a$ | $b$ | $c$ | $\alpha = \beta = \gamma$ |
| 3.186820 | 5.610348 | 29.361165 | 90° |
| Fractional atomic coordinates | | | |
| Atom | $x$ | $y$ | $z$ |
| $S_1$ | 0.0000000000 | 0.2019525010 | 0.1778350410 |
| $S_2$ | 0.5000000000 | 0.6950228301 | 0.1644265681 |
| $S_3$ | 0.0000000000 | 0.8704443839 | 0.2834061530 |
| $S_4$ | 0.5000000000 | 0.3632740326 | 0.2701882807 |
| $S_5$ | 0.0000000000 | 0.2107407693 | 0.3837844005 |
| $S_6$ | 0.5000000000 | 0.7096490634 | 0.3839727777 |
| $S_7$ | 0.0000000000 | 0.2101002552 | 0.4901822977 |
| $S_8$ | 0.5000000000 | 0.7103477769 | 0.4901635849 |
| $W_1$ | 0.5000000000 | 0.9826071337 | 0.2263192516 |
| $W_2$ | 0.0000000000 | 0.5825208141 | 0.2218474430 |
| $W_3$ | 0.5000000000 | 0.3776055328 | 0.4369822265 |
| $W_4$ | 0.0000000000 | 0.8778932018 | 0.4369243734 |

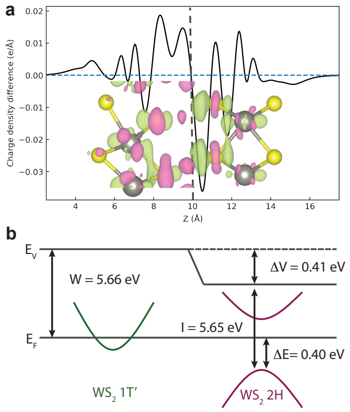


FIG. S2: (a) Plane-averaged charge density difference between the HPB and free-standing 2H and 1T′ monolayer components. Inert: the isosurface of the charge density difference. Purple and green indicate the election gain and loss respectively. (b) Band alignment of the HPB. Green and purple lines represent the metallic and semiconducting band structures of 1T′- and 2H-$WS_2$, respectively.

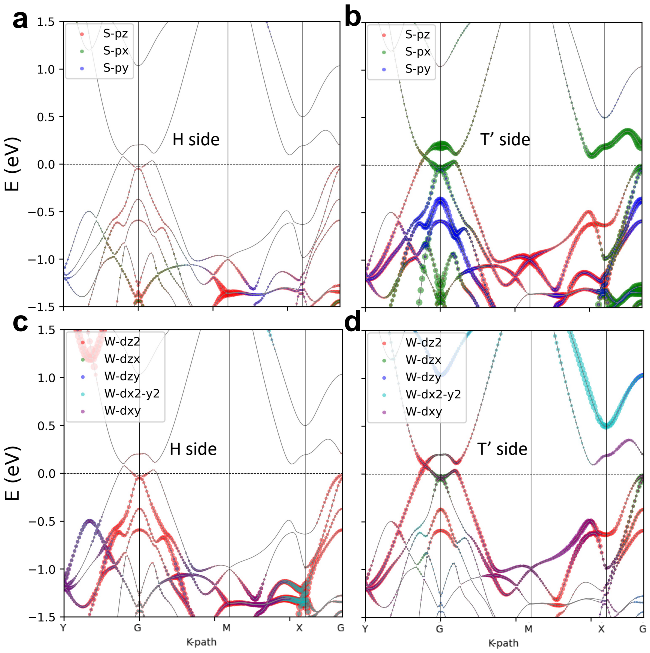


FIG. S3: Orbitals projection of HPB band structure: S $3p$ orbitals on the 2H (a) and 1T$'$ (b) side; W $5d$ orbitals on the 2H (c) and 1T$'$ (d) side.

## II. MODEL HAMILTONIAN

We start from the four band $k \cdot p$ model Hamiltonian for 1T′ monolayer TMDCs,

$$H_{1T'} = \begin{pmatrix} H_1 & V_2 \\ V_1^\dagger & H_2 \end{pmatrix} = \begin{pmatrix} \delta_1 + \frac{\hbar^2 k_x^2}{2m_{1x}} + \frac{\hbar^2 k_y^2}{2m_{1y}} & \lambda_1 (k_y + ik_x) & -iv_{12x}k_x & v_{12y}k_y \\ \lambda_1 (k_y - ik_x) & \delta_1 + \frac{\hbar^2 k_x^2}{2m_{1x}} + \frac{\hbar^2 k_y^2}{2m_{1y}} & v_{12y}k_y & -iv_{12x}k_x \\ iv_{12x}k_x & v_{12y}k_y & \delta_2 + \frac{\hbar^2 k_x^2}{2m_{2x}} + \frac{\hbar^2 k_y^2}{2m_{2y}} & \lambda_2 (k_y + ik_x) \\ v_{12y}k_y & iv_{12x}k_x & \lambda_2 (k_y - ik_x) & \delta_2 + \frac{\hbar^2 k_x^2}{2m_{2x}} + \frac{\hbar^2 k_y^2}{2m_{2y}} \end{pmatrix}. \quad \text{(S1)}$$

With a properly chosen initial guess for these parameters, the model Hamiltonian qualitatively reproduces the the $d-p$ band inversion. However, the orbital projected band structure of the HPB indicates that there is an extra 2H and 1T′ hybridized band near the Fermi level with $d$-orbital-like symmetry. Then an extra 2 x 2 block is introduced in the diagonal of $H_{1T'}$, together with necessary off-diagonal terms, to represent an additional W 5$d$ orbital as shown in the main text. This modified model Hamiltonian has three orbitals, i.e. a six-band model after taking into account the freedom of spin.

First, we consider the simple case when the spin-orbit coupling (SOC) is turned off. The six-band Hamiltonian is given by

$$H_{6b}^0 = \begin{pmatrix} H_1 & 0 & 0 \\ 0 & H_2 & D \\ 0 & D & H_3 \end{pmatrix}, \quad \text{(S2)}$$

where $H_j = \delta_j + \frac{\hbar^2 k_x^2}{2m_{jx}} + \frac{\hbar^2 k_y^2}{2m_{jy}}$ are Hamiltonians of S's $p$ and two W's $d$ orbitals with renormalized mass $m_{jx,y}$. $D = d\mathbb{I}$ is the coupling term between two $d$ bands. The SOC effects of the system can be captured by two extra terms,

$$H_{SOC} = H_{SOC}^1 + H_{SOC}^2 = \begin{pmatrix} 0 & V_2 & V_3 \\ V_1^\dagger & 0 & 0 \\ V_3^\dagger & 0 & 0 \end{pmatrix} + \begin{pmatrix} H_{R1} & 0 & 0 \\ 0 & H_{R2} & 0 \\ 0 & 0 & H_{R3} \end{pmatrix}, \quad \text{(S3)}$$

where $V_j = -iv_{jx}\mathbb{I}k_x + v_{jy}\sigma_x k_y$ and $H_{Rj} = \lambda_j(\sigma_x k_y - \sigma_y k_x)$. $H_{SOC}^1$ is from the monolayer 1T′-$WS_2$, which preserves the inversion and mirror symmetry. $H_{SOC}^2$ is the Rashba SOC under the broken inversion symmetry due to the heterophase stacking.

Parameters of $H_{6b} = H_{6b}^0 + H_{SOC}$ are optimized using the Nelder-Mead method to fit the 6 bands at high symmetry lines near the Fermi level generated by the 44-orbital tight-bind model. To better reproduce the Fermi pockets, the fitting priority is given to the Fermi energy by multiplying a Gaussian function, $G(E) = G_0 e^{(E-E_{Fermi})^2/\sigma}$ to the target function.

TABLE SII: $k \cdot p$ parameters for the HPB $WS_2$

| | | | |
|---|---|---|---|
| $\delta_1(meV)$ | -55 | $\lambda_1(meV\AA)$ | -16 |
| $\delta_2(meV)$ | 186 | $\lambda_2(meV\AA)$ | 25 |
| $\delta_3(meV)$ | 70 | $\lambda_3(meV\AA)$ | -485 |
| $m_{1x}(m_e)$ | 22.65 | $v_{2x}(meV\AA)$ | 918 |
| $m_{1y}(m_e)$ | 1.37 | $v_{2y}(meV\AA)$ | 346 |
| $m_{2x}(m_e)$ | -4.11 | $v_{3x}(meV\AA)$ | 836 |
| $m_{2y}(m_e)$ | -1.37 | $v_{3y}(meV\AA)$ | 208 |
| $m_{3x}(m_e)$ | -0.08 | $d(meV)$ | -86 |
| $m_{3y}(m_e)$ | -0.22 | | |

The low-energy $H_{6b}$ (red) and DFT (black) band structures are compared in Figs. S4 and S5a. The $H_{6b}$ band structure fits well the DFT results within an energy window from -0.04 to 0.04 eV. Without SOC, spin degenerate bands cross along $\Gamma - Y$ and $\Gamma - M$ lines (Fig. S4a). $H_{SOC}^1$ opens up the topological gap (Fig. S4b) and $H_{SOC}^2$ breaks the spin degeneracy and causes Rashba band splitting (Fig. S4c). The Rashba band splitting may close the gap and induce topological phase transition. However, with the optimized parameters, the Rashba band splitting in the $WS_2$ HPB is small compared to the band gap. Therefore the $Z_2$ topological invariant from the monolayer $p-d$ band inversion is preserved in the HPB.

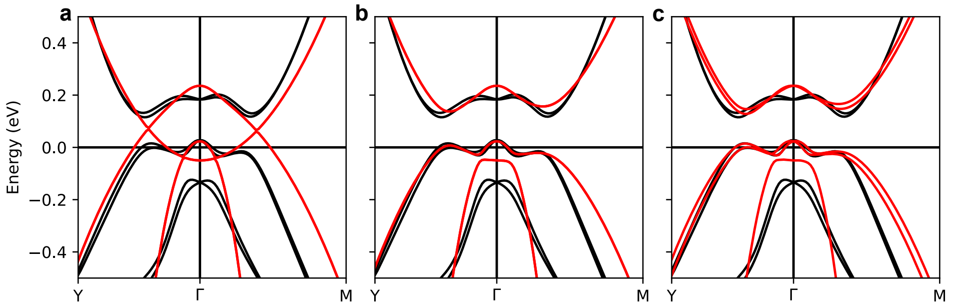


FIG. S4: Low-energy band structure comparison between DFT (black lines) and the $k \cdot p$ model fitting (red lines) without SOC (a), with $H^1_{SOC}$ only (b), and with the full SOC Hamiltonian (c).

To validate the topological properties of the six-bands model Hamiltonian, we compare its Berry curvature with *ab initio* results (Fig. S5b,c). The *ab initio* Berry curvature of the bands are calculated using the Wannier Berri package [11] based on the tight-binding model with 44 maximally localized Wannier basis functions. The Berry curvature of the model Hamiltonian is calculated with the multiband Berry curvature formula,

$$\Omega_n^{ij}(\mathbf{k}) = -2\mathrm{Im}\sum_{m\neq n}\frac{\langle u_n(\mathbf{k})|\frac{\partial \hat{H}}{\partial k_i}|u_m(\mathbf{k})\rangle\langle u_m(\mathbf{k})|\frac{\partial \hat{H}}{\partial k_j}|u_n(\mathbf{k})\rangle}{(\epsilon_n(\mathbf{k})-\epsilon_m(\mathbf{k}))^2}. \tag{S4}$$

The red and blue colors indicate the sign of the Berry curvature. The Berry curvature of $H_{6b}$ is consistent with *ab initio* results, especially in regions where the sign of the Berry curvature flips.

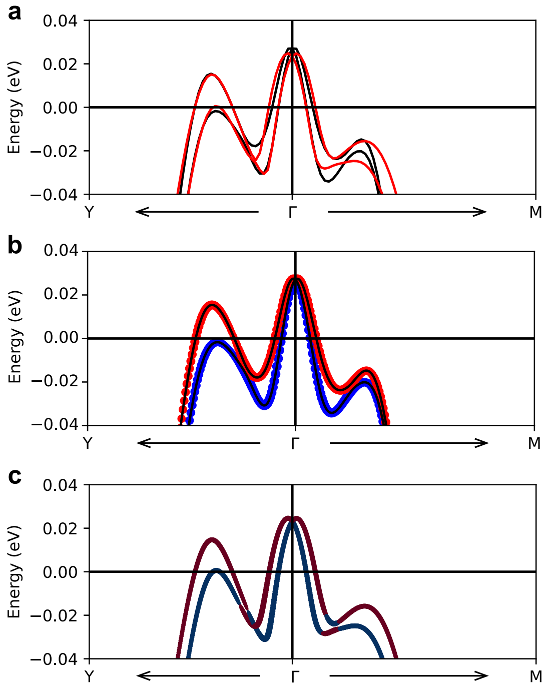


FIG. S5: (a) The low-energy HPB band structure (black) fitting with the six-band $k \cdot p$ model Hamiltonian (red). Berry curvature computed from the tight-binding model (b) and the six-band model Hamiltonian (c). The red and blue color indicate the sign of the Berry curvature. The dot size indicates the magnitude of the Berry curvature in the logarithm scale.

## III. PARTICLE-PARTICLE SUSCEPTIBILITY

### A. General formula

The particle-particle susceptibility for a generic band structure can be expressed as,

$$\Pi(\boldsymbol{q}, \imath\Omega) = \frac{1}{\beta}\sum_{\imath\omega}\int \frac{d^2\boldsymbol{k}}{(2\pi)^2}\mathrm{Tr}[G_\uparrow(\imath\omega + \imath\Omega, \boldsymbol{k}+\boldsymbol{q})G_\downarrow(-\imath\omega, -\boldsymbol{k})] \tag{S5}$$

where $\Omega = 2\pi n/\beta$ are the bosonic frequencies. The Green's function with spin $\sigma =\uparrow, \downarrow$ is given by

$$G_\sigma(\imath\omega, \boldsymbol{k}) = \frac{|u_\sigma(\boldsymbol{k})\rangle\langle u_\sigma(\boldsymbol{k})|}{\imath\omega - \xi_\sigma(\boldsymbol{k})}, \tag{S6}$$

where $\xi(\boldsymbol{k}) = \epsilon_{\boldsymbol{k}} - \mu$ and $u_\sigma(\boldsymbol{k})$ denotes the Bloch wavefunction. By substituting Eq. S6 into Eq. S5, the particle-particle susceptibility becomes

$$\Pi(\boldsymbol{q}, \imath\Omega) = \frac{1}{\beta}\sum_{\imath\omega}\int \frac{d^2\boldsymbol{k}}{(2\pi)^2}\frac{|\langle u_\uparrow(\boldsymbol{k}+\boldsymbol{q})|u_\downarrow(-\boldsymbol{k})\rangle|^2}{(\imath\omega + \imath\Omega - \xi_\uparrow(\boldsymbol{k}+\boldsymbol{q}))(-\imath\omega - \xi_\downarrow(-\boldsymbol{k}))}. \tag{S7}$$

Using the contour method, we can write

$$\Pi(\boldsymbol{q}, \imath\Omega) = -\int \frac{d^2\boldsymbol{k}}{(2\pi)^2}\int_{C'}\frac{dz}{2\pi\imath}n_F(z)\frac{|\langle u_\uparrow(\boldsymbol{k}+\boldsymbol{q})|u_\downarrow(-\boldsymbol{k})\rangle|^2}{(z + \imath\Omega - \xi_\uparrow(\boldsymbol{k}+\boldsymbol{q}))(z + \xi_\downarrow(-\boldsymbol{k}))}, \tag{S8}$$

where the contour $C'$ runs counterclockwise over the poles or branch cuts on the x-axis (or real part of $z$), and $n_F(z)$ is the Fermi-Dirac distribution. Performing the contour integral gives

$$\Pi(\boldsymbol{q}, \imath\Omega) = \int \frac{d^2\boldsymbol{k}}{(2\pi)^2}\left[\frac{n_F(\xi_\uparrow(\boldsymbol{k}+\boldsymbol{q}) - \imath\Omega)}{-\imath\Omega + \xi_\uparrow(\boldsymbol{k}+\boldsymbol{q}) + \xi_\downarrow(-\boldsymbol{k})} + \frac{n_F(-\xi_\downarrow(-\boldsymbol{k}))}{\imath\Omega - \xi_\uparrow(\boldsymbol{k}+\boldsymbol{q}) - \xi_\downarrow(-\boldsymbol{k})}\right]|\langle u_\uparrow(\boldsymbol{k}+\boldsymbol{q})|u_\downarrow(-\boldsymbol{k})\rangle|^2. \tag{S9}$$

Note that we have not assumed time reversal or inversion symmetry since these conditions will generally not be satisfied if the superconducting diode effect is to be realized. Performing analytic continuation to the real axis, $\imath\Omega \to \Omega + \imath\eta$ and $n_F(\epsilon - \imath\Omega) = n_F(\epsilon)$ and $n_F(-\epsilon) = 1 - n_F(\epsilon)$, one gets

$$\Pi(\boldsymbol{q}, \Omega) = \int \frac{d^2\boldsymbol{k}}{(2\pi)^2}\left[\frac{1 - n_F(\xi_\uparrow(\boldsymbol{k}+\boldsymbol{q})) - n_F(\xi_\downarrow(-\boldsymbol{k}))}{-\Omega + (\xi_\uparrow(\boldsymbol{k}+\boldsymbol{q}) + \xi_\downarrow(-\boldsymbol{k})) - \imath\eta}\right]|\langle u_\uparrow(\boldsymbol{k}+\boldsymbol{q})|u_\downarrow(-\boldsymbol{k})\rangle|^2. \tag{S10}$$

The real and imaginary parts of $\Pi(\boldsymbol{q}, \imath\Omega)$ are related to each other by the Kramer-Kronig relations,

$$\mathrm{Re}\Pi(\boldsymbol{q}, \Omega) = \int \frac{d^2\boldsymbol{k}}{(2\pi)^2}\left[\frac{1 - n_F(\xi_\uparrow(\boldsymbol{k}+\boldsymbol{q})) - n_F(\xi_\downarrow(-\boldsymbol{k}))}{-\Omega + (\xi_\uparrow(\boldsymbol{k}+\boldsymbol{q}) + \xi_\downarrow(-\boldsymbol{k}))}\right]|\langle u_\uparrow(\boldsymbol{k}+\boldsymbol{q})|u_\downarrow(-\boldsymbol{k})\rangle|^2, \tag{S11}$$

$$\mathrm{Im}\Pi(\boldsymbol{q}, \imath\Omega) = \int \frac{d^2\boldsymbol{k}}{(2\pi)^2}\frac{1}{\pi}[1 - n_F(\xi_\uparrow(\boldsymbol{k}+\boldsymbol{q})) - n_F(\xi_\downarrow(-\boldsymbol{k}))]\delta(\Omega - (\xi_\uparrow(\boldsymbol{k}+\boldsymbol{q}) + \xi_\downarrow(-\boldsymbol{k}))) \\ |\langle u_\uparrow(\boldsymbol{k}+\boldsymbol{q})|u_\downarrow(-\boldsymbol{k})\rangle|^2. \tag{S12}$$

### B. Rashba electron gas

In the Rahsba electron gas, the spin is no longer a good quantum number. Thus, we denote the split bands with the $\pm$ sign. Therefore, we have

$$\Pi(\boldsymbol{q}, \Omega)_{\alpha\beta} = \int \frac{d^2\boldsymbol{k}}{(2\pi)^2}\left[\frac{1 - n_F(\xi_\alpha(\boldsymbol{k}+\boldsymbol{q})) - n_F(\xi_\beta(-\boldsymbol{k}))}{-\Omega + (\xi_\alpha(\boldsymbol{k}+\boldsymbol{q}) + \xi_\beta(-\boldsymbol{k})) - \imath\eta}\right]|\langle u_\alpha(\boldsymbol{k}+\boldsymbol{q})|u_{\beta\mathcal{T}}(-\boldsymbol{k})\rangle|^2, \tag{S13}$$

where $\alpha, \beta = \pm$ and $u_{\beta\mathcal{T}}$ is the time reversal pair of $u_\beta$, i.e. $u_{\beta\mathcal{T}} = i\sigma_y\mathcal{K}u_\beta$. The Rashba electron gas Hamiltonian is given by

$$H_R = \frac{\hbar k^2}{2m} - \mu + \lambda(\vec{\sigma}\times\vec{k})\cdot\vec{z}, \tag{S14}$$

whose eigenvalues and eigenstates are

$$\xi_\pm(k) = \frac{\hbar k^2}{2m} \pm \lambda\sqrt{k_x^2 + k_y^2}, \tag{S15}$$

$$|u_+\rangle = \frac{1}{\sqrt{2}}\begin{pmatrix} 1 \\ e^{i\varphi_k} \end{pmatrix}, \tag{S16}$$

$$|u_-\rangle = \frac{1}{\sqrt{2}}\begin{pmatrix} 1 \\ -e^{i\varphi_k} \end{pmatrix}, \tag{S17}$$

where $k_x = k\cos\varphi_k, k_y = k\sin\varphi_k$. This leads to

$$\langle u_\pm(\boldsymbol{k}+\boldsymbol{q})|u_{\pm\mathcal{T}}(-\boldsymbol{k})\rangle = \frac{1}{2}(\pm e^{-i\varphi_{k+q}} \mp e^{-i\varphi_{-k}}), \tag{S18}$$

$$\langle u_\pm(\boldsymbol{k}+\boldsymbol{q})|u_{\mp\mathcal{T}}(-\boldsymbol{k})\rangle = \frac{1}{2}(\pm e^{-i\varphi_{k+q}} \pm e^{-i\varphi_{-k}}). \tag{S19}$$

The expressions of $\Pi(\boldsymbol{q}, \Omega$ are given by

$$\Pi(\boldsymbol{q},\Omega)_{\pm\pm} = \int \frac{d^2\boldsymbol{k}}{(2\pi)^2}\left[\frac{1 - n_F(\xi_\pm(\boldsymbol{k}+\boldsymbol{q})) - n_F(\xi_\pm(-\boldsymbol{k}))}{-\Omega + (\xi_\pm(\boldsymbol{k}+\boldsymbol{q}) + \xi_\pm(-\boldsymbol{k})) - \imath\eta}\right]\sin^2\frac{\varphi_{k+q} - \varphi_{-k}}{2}, \tag{S20}$$

$$\Pi(\boldsymbol{q},\Omega)_{\pm\mp} = \int \frac{d^2\boldsymbol{k}}{(2\pi)^2}\left[\frac{1 - n_F(\xi_\pm(\boldsymbol{k}+\boldsymbol{q})) - n_F(\xi_\mp(-\boldsymbol{k}))}{-\Omega + (\xi_\pm(\boldsymbol{k}+\boldsymbol{q}) + \xi_\mp(-\boldsymbol{k})) - \imath\eta}\right]\cos^2\frac{\varphi_{k+q} - \varphi_{-k}}{2}. \tag{S21}$$

### C. Rashba electron gas in a magnetic field

When a magnetic field is applied, the Zeeman term is added to the Rashba Hamiltonian,

$$H = \frac{\hbar k^2}{2m} - \mu + \lambda(\vec{\sigma}\times\vec{k})\cdot\vec{z} - \vec{B}\cdot\vec{\sigma} \tag{S22}$$

Assuming the $\vec{B}$ is in-plane along the $x$ direction, we have

$$H = \frac{\hbar k^2}{2m} - \mu + \lambda(\vec{\sigma}\times\vec{k})\cdot\vec{z} - B_x\sigma_x - B_y\sigma_y \tag{S23}$$

with eigenvalues and eigenstates,

$$\xi_\pm(k) = \frac{\hbar k^2}{2m} \pm \sqrt{(\lambda k_x - B_x)^2 + (\lambda k_y - B_y)^2}, \tag{S24}$$

$$|u_+\rangle = \frac{1}{\sqrt{2}}\begin{pmatrix} 1 \\ e^{i\varphi_k(B)} \end{pmatrix}, \tag{S25}$$

$$|u_-\rangle = \frac{1}{\sqrt{2}}\begin{pmatrix} 1 \\ -e^{i\varphi_k(B)} \end{pmatrix}, \tag{S26}$$

where $\varphi_k(B) = \arctan\frac{\lambda k_x - B_x}{\lambda k_y - B_y}$. Therefore, the particle-particle susceptibility can be written as,

$$\Pi(\boldsymbol{q},\Omega)_{\pm\pm} = \int \frac{d^2\boldsymbol{k}}{(2\pi)^2}\left[\frac{1 - n_F(\xi_\pm(\boldsymbol{k}+\boldsymbol{q})) - n_F(\xi_\pm(-\boldsymbol{k}))}{-\Omega + (\xi_\pm(\boldsymbol{k}+\boldsymbol{q}) + \xi_\pm(-\boldsymbol{k})) - \imath\eta}\right]\sin^2\frac{\varphi_{k+q}(B) - \varphi_{-k}(B)}{2}, \tag{S27}$$

$$\Pi(\boldsymbol{q},\Omega)_{\pm\mp} = \int \frac{d^2\boldsymbol{k}}{(2\pi)^2}\left[\frac{1 - n_F(\xi_\pm(\boldsymbol{k}+\boldsymbol{q})) - n_F(\xi_\mp(-\boldsymbol{k}))}{-\Omega + (\xi_\pm(\boldsymbol{k}+\boldsymbol{q}) + \xi_\mp(-\boldsymbol{k})) - \imath\eta}\right]\cos^2\frac{\varphi_{k+q}(B) - \varphi_{-k}(B)}{2}, \tag{S28}$$

Numerical calculations of the total particle pair susceptibly show that the peak shifts to positive and negative $q$ due to inner and outer Rashba Fermi pocket pairing as the magnetic Zeeman energy $B$ increases, where the Rashba SOC strength $\lambda$ is set as 0.1, $\frac{\hbar}{2m} = \mu = 1$ and $\beta = 1/0.0001$. The difference in peak heights at positive and negative $q$'s is caused by the difference of the Fermi density of state of inner and outer pockets.

### D. Heterophase bilayer model Hamiltonian

In the six-band model Hamiltonian, we focus on the middle two bands (labeled with the $\pm$ sign) that are near the Fermi level. The eigenstates $u_\alpha$ and eigenvalues $\xi_\alpha$ of the $\pm$ bands are solved numerically. Next, the pair susceptibility is calculated using Eq. 5 in the main text. We sample the center Brillouin zone with dense $2000\times4000$ k point mesh. The q value are chosen to be the integer multiples of $\Delta k$, which yields

$$\Pi(\boldsymbol{q},\Omega)_{\alpha\beta} = \sum_{\boldsymbol{k}} \frac{(\Delta \boldsymbol{k})^2}{(2\pi)^2}\left[\frac{1-n_F(\xi_\alpha(\boldsymbol{k}+\boldsymbol{q}))-n_F(\xi_\beta(-\boldsymbol{k}))}{-\Omega-(\xi_\alpha(\boldsymbol{k}+\boldsymbol{q})+\xi_\beta(-\boldsymbol{k}))-\imath\eta}\right]|\langle u_\alpha(\boldsymbol{k}+\boldsymbol{q})|u_{\beta\mathcal{T}}(-\boldsymbol{k})\rangle|^2. \tag{S29}$$

In the main text, we consider the static susceptibility and set $\Omega = 0$. $\eta$ is set to a small value $10^{-7}$.

## IV. PHONON DRIVEN SUPERCONDUCTIVITY IN THE $WS_2$ HPB

Since bulk 1T′-$WS_2$ is known as a conventional phonon-driven superconductor, we first calculate the phonon dispersion of the $WS_2$ HPB and compare it to the monolayer 1T′-$WS_2$ as shown in Fig. S6. The 2H side and 1T′ side dominated modes are shown in purple and green colors, respectively. We find that the phonon bands are separated as the 1T′ and 2H regions with only a few hybridizations at the acoustic and optical phonon bands minimum. The 2H phase phonon strongly enhances the phonon density of states near the 40 meV region as shown in Fig. S6c. The shadow region is the phonon DOS of HPB while the green line is that of the monolayer. Moreover, there is no imaginary phonon mode in the HPB, which confirms the HPB model is stable.

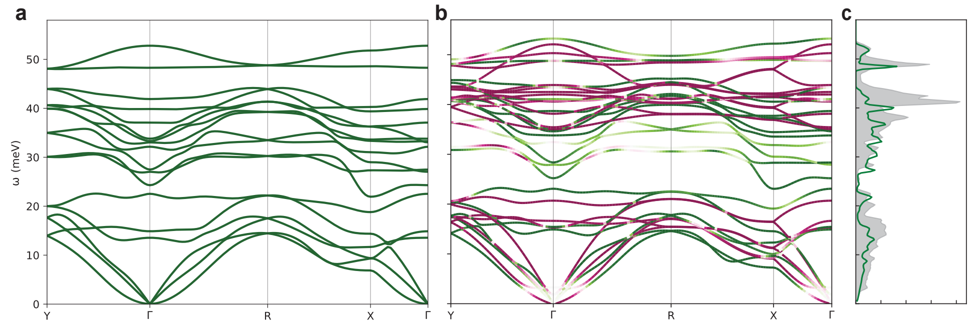


FIG. S6: The phonon dispersion of monolayer 1T′-$WS_2$ (a) and HPB $WS_2$ (b). Purple and green indicate the projection on the 2H and 1T′ phase components respectively. (c) Phonon DOS of the monolayer (green) and HPB (shadowed).

The electron DOS of 1T′-$WS_2$ bilayer, HPB and 1T′-$WS_2$ monolayer sampled with fine K-point grids are shown in Fig. S7. The bilayer has the largest Fermi DOS, while HPB is between the bilayer and monolayer, which is consistent with Fermi pocket plots. In Fig. S8, we plot the phonon DOS and electron-phonon properties including isotropic Eliashberg spectral function $\alpha^2F(\omega)$ and the cumulated $\lambda(\omega) = 2\int_0^\omega \alpha^2F(\omega)\omega\mathrm{d}/\omega$ of bilayer, HPB and monolayer. The EPC strengths are listed in Table SIII. We find that the bilayer has the largest EPC strength $\lambda$ and the HPB is between the bilayer and monolayer. Comparing $\alpha^2F(\omega)$ of the HPB and monolayer, the main contributions of the 2H phase phonon modes are located at approximately 40 meV in the HPB and they do not significantly contribute to the electron-phonon coupling. Therefore, the larger Fermi DOS rather than the phonon modes from the 2H phase enhances the EPC in HPB relative to the monolayer.

We calculate the superconducting temperatures ($T_C$) of 1T′-$WS_2$ bilayer, HPB and 1T′-$WS_2$ monolayer using the Allen-Dynes formula (ref),

$$T_c = \frac{\omega_{\log}}{1.2}\exp\left(\frac{-1.04(1+\lambda)}{\lambda-\mu^*(1+0.62\lambda)}\right), \tag{S30}$$

where the screened Coulomb potential $\mu^*$ is set as 0.1. The results are summarized in Table SIII. As a comparison, the $T_C$ of bulk 1T′-$WS_2$ is also calculated to be 7.9 K, which is consistent with the previous result of 8.5 K [12] and experimental measurement of 8.6 K [13]. Calculated $T_C$ of the monolayer appears to be lower than the experimental measurement of 5.7 K [13]. The 1T-WS2 monolayer may be doped by the substrate, which will enhance its $T_c$. Overall, the trend that $T_c$ increases from monolayer to bulk is very well captured by our calculation. Calculated $T_C$ of the HPB is 1.1 K, which lies between the bilayer and monolayer.

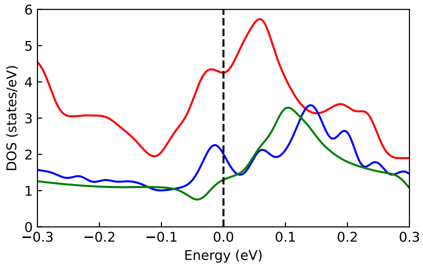


FIG. S7: The electron DOS of the bilayer (red), HPB (blue) and monolayer (green).

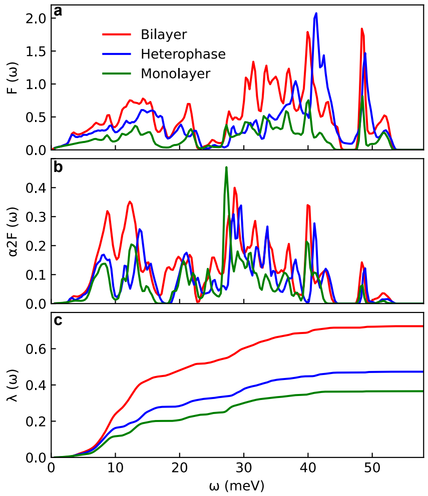


FIG. S8: (a) Phonon DOS, (b) the isotropic Eliashberg spectral function and (c) EPC strength of the bilayer (red), HPB (blue) and monolayer (green).

TABLE SIII: $T_c$ of the $WS_2$ systems. Values in the parentheses are taken from the literature.

| | Bulk | Bilayer | HPB | Monolayer |
|---|---|---|---|---|
| $T_c$(K) | 7.9 (8.5$^a$, 8.6$^b$ and 8.8$^c$) | 6.3 (7$^a$) | 1.1 | 0.4 (5.7$^b$) |

$^a$ simulation [12], $^b$ experiment [13]. $^c$ experiment [14].

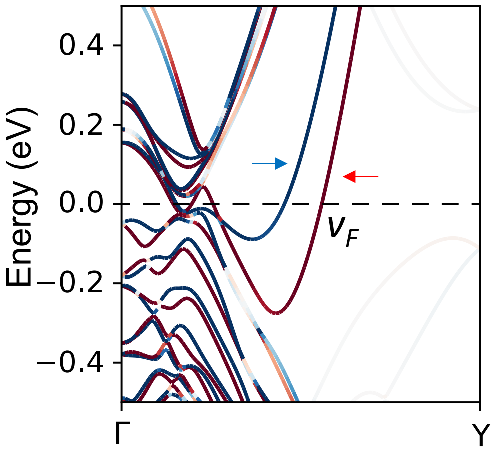


FIG. S9: Tight-binding band structure of the $WS_2$ HPB ribbon under zero field. Edge states are indicated by arrows (red: spin up; blue: spin down).

[1] P. Giannozzi *et al.*, Quantum espresso: a modular and open-source software project for quantum simulations of materials, Journal of Physics: Condensed Matter **21**, 395502 (2009).

[2] M. Setten, The pseudodojo: training and grading a 85 element optimized norm-conserving pseudopotential table, Comput. Phys. Commun. **226**, 10.1016/j.cpc.2018.01.012 (2018).

[3] J. P. Perdew, K. Burke, and M. Ernzerhof, Generalized gradient approximation made simple, Physical Review Letters **77**, 3865 (1996).

[4] S. Grimme, J. Antony, S. Ehrlich, and H. Krieg, A consistent and accurate ab initio parametrization of density functional dispersion correction (dft-d) for the 94 elements h-pu, Journal of Chemical Physics **132**, 154104 (2010).

[5] T. Sohier, M. Calandra, and F. Mauri, Density functional perturbation theory for gated two-dimensional heterostructures: Theoretical developments and application to flexural phonons in graphene, Physical Review B **96**, 075448 (2017).

[6] N. Marzari, A. A. Mostofi, J. R. Yates, I. Souza, and D. Vanderbilt, Maximally localized wannier functions: Theory and applications, Reviews of Modern Physics **84**, 1419 (2012).

[7] G. Pizzi *et al.*, Wannier90 as a community code: New features and applications, Journal of Physics: Condensed Matter **32**, 165902 (2020).

[8] F. Giustino, M. L. Cohen, and S. G. Louie, Electron-phonon interaction using wannier functions, Physical Review B: Condensed Matter and Materials Physics **76**, 165108 (2007).

[9] S. Poncé, E. R. Margine, C. Verdi, and F. Giustino, Epw: Electron-phonon coupling, transport and superconducting properties using maximally localized wannier functions, Computer Physics Communications **209**, 116 (2016).

[10] Q. Wu, S. Zhang, H. F. Song, M. Troyer, and A. A. Soluyanov, Wanniertools: an open-source software package for novel topological materials, Comput. Phys. Commun. **224**, 10.1016/j.cpc.2017.09.033 (2018).

[11] S. S. Tsirkin, High performance wannier interpolation of berry curvature and related quantities with wannierberri code, npj Computational Materials **7**, 33 (2021).

[12] C.-S. Lian, C. Si, and W. Duan, Anisotropic full-gap superconductivity in 2m-ws2 topological metal with intrinsic proximity effect, Nano Letters **21**, 709 (2020).

[13] Z. Lai, Q. He, T. H. Tran, D. M. Repaka, D.-D. Zhou, Y. Sun, S. Xi, Y. Li, A. Chaturvedi, C. Tan, *et al.*, Metastable 1t-phase group vib transition metal dichalcogenide crystals, Nature Materials **20**, 1113 (2021).

[14] Y. Fang, J. Pan, D. Zhang, D. Wang, H. T. Hirose, T. Terashima, S. Uji, Y. Yuan, W. Li, Z. Tian, *et al.*, Discovery of superconductivity in 2m ws2 with possible topological surface states, Advanced Materials **31**, 1901942 (2019).
